# Supplementary material for: Multi-Agent Contract Design: How to Commission Multiple Agents with Individual Outcome
Source: arXiv:2301.13654 source file (2023-01-31)
Supplement: Supplementary file 7 [file appendixHardness.tex]

%\section{Proofs Omitted from Section~\ref{sec:hard} }




%\subsection{Hardness Result of~\textsc{ApxCPE}}

\section{Proofs Omitted from Section~\ref{sec:hard}}

\theoremHardness*

\begin{proof}
We reduce from \textsc{GAP-INDEPENDENT-SET}, which is a promise problem that formally reads as follows: given an $\delta > 0$ and a graph $G= (V,E)$, with set of nodes $V$ and set of edges $E$, determine whether $G$ admits an independent set of size at least $|V|^{1-\delta}$ or all the independent sets of $G$ have size smaller than $|V|^{\delta}$. 
\textsc{GAP-INDEPENDENT-SET} is \NPHard\ for every $\delta>0$~\citep{hastad1999clique,Zuckerman2007linear}.

 Let $\ell=|V|$ and $\alpha>0$ be the desired approximation factor. Given an instance of \textsc{GAP-INDEPENDENT-SET}, we build an instance such that if there exists an independent set of size $\ell^{1-\delta}$, then there exists a Constrained Phi-equilibrium with social welfare 1.
Otherwise, if all the independent sets have size at most $\ell^\delta$, all the Constrained $\epsilon$-Phi-equilibria have social welfare at most $\alpha/2$.
We can use any $\delta>0$, since we simply need $\ell^\delta<\ell^{1-\delta}$.
Moreover, we take $\epsilon=\frac{\alpha^2}{128 \ell^2}$. As we will see,  $\ell$ will be smaller than the number of action of the players, satisfying the condition in the statement.
	\paragraph{Construction.} 
	The first player has a set of actions $\A_1$ that includes actions $a_0$, $a_1$, $a_2$ and an action $a_v$ for each $v \in V$. Moreover, the first player has an action $a_F$.\footnote{This action is needed only to satisfy the strictly feasibility assumption.} 
	The second player has a set of actions $\A_2$ that includes actions $a_v$ and $\bar a_{v}$ for each $v \in V$. Moreover, the second player has an action $a_F$. 
	Let $\gamma=\eta=\alpha/8$.
	The utility of the first agent is as follows:
	\begin{itemize}
	\item $u_1(a_0,a)=\gamma+\frac{1}{2}\eta$ for all $a \in \A_2 \setminus \{a_F\}$,
	\item $u_1(a_1,a_v)=\gamma+\eta$ and $u_1(a_2,a_v)=\gamma$ for all $v \in V$.
	 \item $u_1(a_1,\bar a_v)=\gamma$ and $u_1(a_2,\bar a_v)=\gamma+\eta$ for all $v \in V$.
	 \item $u_1(a_v, a_{v})=u_1(a_v,\bar a_{v})=\gamma$ for all $v \in V$
	 \item $u_1(a_{v}, a_{v'})=\gamma$ and  $u_1(a_{v},\bar a_{v'})=\gamma+\frac{\ell-\ell^{1-\delta}}{\ell-\ell^{1-\delta}-1}\eta$ for all $v'\neq v$.
	 \item $u_1(a_F,a)=0$ for each $a \in \A_2$.
	 	 \item $u_1(a,a_F)=0$ for each $a \in \A_1$.
 	 \end{itemize}
 	The utility of the second agent is $u^2(a_0,a)=1$ for each $a \in \A_2 \setminus \{a_F\}$ and $0$ otherwise.
	 
	 There is a cost function $c_v$ for each $v \in V$, which is common to both the agents.
	 For each $v \in V$, the cost function $c_v$ is such that
	 \begin{itemize}
	 	\item $c_v(a_v, a_{v'})=-1$ for each $v'\neq v$, $(v,v') \in E$, \item $c_v(a_v, a_{v'})=0$ for each $v' \neq v, (v,v') \notin E$, 
	 	\item $c_v(a_v, a_{v})=1$ for each $v \in V$.
	 	\item $c_v(a_F,a)=-\frac{1}{4\ell^2}$ for each $a \in \A_2$. 
	 	\item $c_v(a,a_F)=-\frac{1}{4\ell^2}$ for each $a \in \A_1$.
	 	\item For every other action profile the cost is $0$.
	 \end{itemize}
	We dropped the player index from the cost functions $c$ as they are equal to both players.
 	
 	Moreover, we set of deviations $\Phi_i=\Phi_{i,\textsc{all}}$ for both players $i\in\{1,2\}$.
 	
 	Notice that the instance satisfies Assumption~\ref{ass:strictly}. Indeed, the deviation $\phi_i$ such that $\phi_i[a,a_F]=1$ for all $a\in\A_{i}$ for $i\in\{1,2\}$, that deviates deterministically to $a_F$ is always strictly feasible for both player $1$ and player $2$. Moreover, its cost is polynomial in the instance size.

	
	\paragraph{Completeness.}
	We show that if there exists an independent set of size $\ell^{1-\delta}$, then the social welfare of an optimal Constrained Phi-equilibria is at least $1$.
	Let $V^*$ be an independent set of size $\ell^{1-\delta}$. We build a Constrained Phi-equilibria $\zvec$ with social welfare at least $1$. Consider the correlated strategy such that $\zvec[a_0,a_v]=\frac{1}{2\ell^{1-\delta}}$ for all $v \in V^*$, while $\zvec[a_0,\bar a_v]=\frac{1}{2(\ell-\ell^{1-\delta})}$ for all $v \notin V^*$. All the other action profiles have probability $0$.
	
	It is easy to see that the correlated strategy has social welfare at least $1$ since player $1$ always plays action $a_0$ and $u^2(a_0,a)=1$ for all $a \in \A_2$. Moreover, it is easy to verify that it is safe since $c_v(a_0,a)\le 0$ for each $a \in \A_2$.
	Hence, to show that $z$ is an Constrained Phi-equilibria we only need to prove that it satisfies the incentive constraints.
	The incentive constraints of the second player are satisfied since they obtain the maximum possible utility, \emph{i.e.}, $1$. 
	
	Consider now a possible deviation of the first player $\phi_1\in\Phi_1$.
	As a first step, we compute the expected utility of a strategy $\phi_1$.
	Let us define the following quantities:
	\begin{itemize}
		\item $T^1=\sum_{v \in V^*}  \phi_1[a_0,a_v] \left[ \left(\zvec[a_0,a_v] +\zvec[a_0,\bar a_v] +\sum_{v' \neq v} \zvec[a_0,a_{v'}] \right) \gamma + \left(\gamma +\frac{\ell-\ell^{1-\delta}}{\ell-\ell^{1-\delta}-1}\eta \right) \sum_{v' \neq v}  \zvec[a_0,\bar a_v]          \right] $ 
		\item $T^2=\sum_{v \notin V^*} \phi_1[a_0,a_v] \left[ \left(\zvec[a_0,a_v] +\zvec[a_0,\bar a_v] +\sum_{v' \neq v} \zvec[a_0,a_{v'}] \right) \gamma+ \left(\gamma +\frac{\ell-\ell^{1-\delta}}{\ell-\ell^{1-\delta}-1}\eta\right)  \sum_{v' \neq v}  \zvec[a_0,\bar a_v]          \right] $
		\item  $T^3 = \left(\gamma + \frac{\eta}{2}\right)  \phi_1[a_0,a_0] +  \frac{\gamma + \eta}{2} (\phi_1[a_0,a_1]+\phi_1[a_0,a_2])+ \frac{\gamma}{2} (\phi_1[a_0,a_1]+\phi_1[a_0,a_2]) $
	\end{itemize}

	
	We bound each component individually.
	\begin{align*}
	T^1&=\sum_{v \in V^*}  \phi_1[a_0,a_v] \left[ \left(\zvec[a_0,a_v] +\zvec[a_0,\bar a_v] +\sum_{v' \neq v} \zvec[a_0,a_{v'}] \right)\gamma+  \left(\gamma + \eta\frac{\ell-\ell^{1-\delta}}{\ell-\ell^{1-\delta}-1}\right) \sum_{v' \neq v}  \zvec[a_0,\bar a_v]          \right] \\
	&=\sum_{v \in V^*}  \phi_1[a_0,a_v] \left[\frac{1}{2}\gamma + \frac{1}{2}\left(\gamma + \eta\frac{\ell-\ell^{1-\delta}}{\ell-\ell^{1-\delta}-1}\right) \right] \\
	&=\sum_{v \in V^*}  \phi_1[a_0,a_v] \left(\gamma+\frac{\eta}{2}\frac{\ell-\ell^{1-\delta}}{\ell-\ell^{1-\delta}-1}\right) \\
	&\le \sum_{v \in V^*}  \phi_1[a_0,a_v] (\gamma+\eta) ,
	\end{align*}
	where in the last inequality we use  $\frac{\ell-\ell^{1-\delta}}{\ell-\ell^{1-\delta}-1}\le 2$ for $\ell$ large enough.
	while
	\begin{align*}
	T^2&=\sum_{v \notin V^*}  \phi_1[a_0,a_v] \left[ \left(\zvec[a_0,a_v] +\zvec[a_0,\bar a_v] +\sum_{v' \neq v} \zvec[a_0,a_{v'}] \right) \gamma + \left(\gamma +\eta\frac{\ell-\ell^{1-\delta}}{\ell-\ell^{1-\delta}-1}  \right) \sum_{v' \neq v}  \zvec[a_0,\bar a_v]          \right] \\
	&= \sum_{v \notin V^*}  \phi_1[a_0,a_v] \left[\left(\frac{1}{2}+\frac{1}{2(\ell-\ell^{1-\delta})}\right)\gamma + \left(\frac{1}{2}-\frac{1}{2(\ell-\ell^{1-\delta})}\right) \left(\gamma +\eta\frac{\ell-\ell^{1-\delta}}{\ell-\ell^{1-\delta}-1} \right)\right]\\
	&=\sum_{v \notin V^*}  \phi_1[a_0,a_v]\left[\gamma +\frac{\eta}{2}\left(\frac{\ell-\ell^{1-\delta}}{\ell-\ell^{1-\delta}-1}-\frac{1}{\ell-\ell^{1-\delta}-1} \right)\right]\\
	&=\sum_{v \notin V^*}  \phi_1[a_0,a_v]\left(\gamma + \frac{\eta}{2}\right).
	\end{align*}
	Finally, 
	\begin{align*}
	T^3& = [a_0,a_0] \left(\gamma + \frac{\eta}{2}\right) + \frac{\gamma + \eta}{2}([a_0,a_1]+[a_0,a_2]) +\frac{\gamma}{2}([a_0,a_1]+[a_0,a_2])  \\
	&= \left( \gamma + \frac{\eta}{2}\right)\left([a_0,a_0] + \phi_1[a_0,a_1]+\phi_1[a_0,a_2]\right)
	\end{align*}
	
	Finally, the utility of a deviation $\phi_1$ is
	\begin{align*}
	&\sum_{a^1 \in \A_1,a^2\in \A_2} \sum_{a \in A_1} \phi_1[a^1,a] \zvec[a^1,a^2] u_1(a,a^2)\\
	&=  \sum_{a \in \A_1,a^2 \in \A_2} \phi_1[a_0,a] \zvec[a_0,a^2]u_1(a,a^2)\\
	&=T^1+T^2+T^3  \\
	&\le (\gamma+\eta) \sum_{v \in V^*}  \phi_1[a_0,a_v]  + \left(\gamma + \frac{\eta}{2} \right) \sum_{v \notin V^*}  \phi_1[a_0,a_v] +\left( \gamma + \frac{\eta}{2}\right)(\phi[a_0,a_0] + \phi_1[a_0,a_1]+\phi_1[a_0,a_2]) \\
	&=\frac{\eta}{2}\sum_{v \in V^*}  \phi_1[a_0,a_v]  +  \left(\gamma +\frac{\eta}{2}\right)(1- \phi_1[a_0,a_F] )
	\end{align*}
	
	Now, we show that no deviation $\phi_1\in\Phi_1$ is both safe and increases player $1$ utility. In particular, we show that if a strategy $\phi_1$ increases the utility than it is not safe.
	Indeed, if $\phi_1$ increases the utility, then
	\begin{align*}
	&\sum_{\substack{a^1 \in \A_1,\\a^2\in \A_2}} \sum_{a \in A_1} \phi_1[a^1,a] \zvec[a^1,a^2] u_1(a,a^2)> \gamma+ \frac{\eta}{2}
	\end{align*}
	This implies that 
		\begin{align*}
	&\frac{\eta}{2}\sum_{v \in V^*}  \phi_1[a_0,a_v]  +   \left(\gamma +\frac{\eta}{2}\right)(1- \phi_1[a_0,a_F] )  > \gamma+ \frac{\eta}{2}
	\end{align*}
	and 
	\begin{align}\label{eq:vLarge}
	&\sum_{v \in V^*}  \phi_1[a_0,a_v]    > \frac{1}{2}  \phi_1[a_0,a_F] 
	\end{align}
	
	
	Next, we show that any $\phi_1$ that increases the utility (and hence that satisfies Eq~\eqref{eq:vLarge}) is not a feasible deviation.
	First, notice that equation~\eqref{eq:vLarge} implies that there is a $\bar v\in V^*$ such that 
	\begin{align} \label{eq:vLarge2}
	&\phi_1[a_0,a_{\bar v}] > \frac{1}{2\ell}   \phi_1[a_0,a_F].
	\end{align}
	Then, we show that the deviation $\phi_1$ violates the constraint $c_{\bar v}$.
	 In particular,
	\begin{align*}
	\sum_{a^1 \in \A_1,a^2\in \A_2} \sum_{a \in \A_1} \phi_1[a^1,a] \zvec[a^1,a^2] c_v(a,a^2)&=  \phi_1[a_0,a_{\bar v}] \zvec[a_0,a_{\bar v}] 1 - \frac{1}{4\ell^2}\phi_1[a_0,a_F] - \sum_{\substack{v \in V^*: (v,\bar v) \in E }} \phi_1[a_0,a_{\bar v}] \zvec[a_0,a_v] 1  \\
	&=  \phi_1[a_0,a_{\bar v}] \zvec[a_0,a_{\bar v}]  - \frac{1}{4\ell^2} \phi_1[a_0,a_F]  \\
	 &=  \frac{1}{2\ell^{1-\frac{1}{\ell}}} \phi_1[a_0,a_{\bar v}]  -\frac{1}{4\ell^2}  \phi_1[a_0,a_F] \\
	&> \phi_1[a_0,a_{\bar v}] \left(\frac{1}{2\ell^{1-\frac{1}{\ell}}} -  \frac{1}{2\ell} \right)   \ge 0,
	\end{align*}
	where the second inequality holds since $V^*$ is an independent set, and the second-to-last inequality by Equation~\eqref{eq:vLarge2}.
	Hence, there is no deviation $\phi_1$ that increases players $1$ utility and that is safe. This concludes the first part of the proof.
	

	
	\textbf{Soundness.} We show that if there exists a Constrained $w$-Phi-equilibria with social welfare $\alpha/2$, then there exists an independent set of size strictly larger than  $\ell^{\delta}$, reaching a contradiction.  
	Suppose by contradiction that there exists a Constrained $\epsilon$-Phi-equilibrium $\zvec$ with social welfare strictly greater than $\alpha/2$. 
	Thus, 
	\[
	\sum_{a' \in \A_2 \setminus \{a_F\}} \zvec[a_0,a'] \cdot1 +\sum_{a \in \A_1,a' \in \A_2} (\gamma+\eta) \ge  \sum_{a \in \A_1,a' \in \A_2} \zvec[a,a'] (u_1(a,a')+u^2(a,a')) \ge \alpha/2,
	\] 
	where the first inequality comes from $u_2(a_0,a')=1$ for each $a'\in \A_2 \setminus \{a_F\}$ and $0$ otherwise, and $u_1(a,a')\le \gamma+\eta$ for each $a\in \A_1$ and $a' \in \A_2$.
	This implies 
	\begin{align}\label{eq:highProb}
	\sum_{a' \in \A_2} \zvec[a_0,a'] \ge \alpha/4.
	\end{align}

  	Then, we show that $\zvec$ assigns similar probabilities on the set of action profiles $\{a_0,a_v\}_{v \in V}$ and $\{a_0,\bar a_v\}_{v \in V}$
	Given an $a \in \A_1$, let $\phi_{a}\in\Phi_1$ be a deviation of the first player such that $\phi_{a}[a_0,a]=1$ and $\phi_{a}[a',a']=1$ for each $a' \neq a_0$.
	Since $\zvec$ is an Constrained $\epsilon$-Phi-equilibrium there is no feasible deviation $\phi_{a}$ that increases the utility of player $1$ by more than $\epsilon$.
	This implies that 
	\begin{align}\label{eq:balance2}
		\left|\sum_{v \in V} \zvec[a_0,a_v]-\sum_{v \in V} \zvec[a_0,\bar a_v]\right|\le \frac{2\epsilon}{\eta}.
	\end{align}
	Indeed, if 
	\begin{align}\label{eq:balance}
		&\sum_{v \in V} \zvec[a_0,a_v]> \sum_{v \in V} \zvec[a_0,\bar a_v]+ \frac{2\epsilon}{\eta},
	\end{align}
	 then the deviation  $\phi_{a_1}$ has utility at least
	\begin{align*}
		\sum_{v \in V} \zvec[a_0,a_v] &\phi_{a_1}[a_0,a_1] (\gamma+\eta) + \zvec[a_0,\bar a_v] \phi_{a_1}[a_0,a_1] \gamma +   \sum_{a \in \A_1 \setminus \{a_0\}} \sum_{ a' \in \A_2} \zvec[a, a'] \phi_{a_1}[a,a] u^i(a, a')\\
		&=  \eta \sum_{v \in V} \zvec[a_0,a_v]  +  \gamma \sum_{v \in V} \left(\zvec[a_0, a_v] + \zvec[a_0,\bar a_v] \right) +   \sum_{a \in \A_1 \setminus \{a_0\}} \sum_{ a' \in \A_2} \zvec[a, a'] \phi_{a_1}[a,a] u^i(a, a')\\
		&> \frac{\eta}{2} \left(\frac{2\epsilon}{\eta}+\sum_{v \in V} (\zvec[a_0,a_v] + \zvec[a_0,\bar a_v])\right)+  \gamma \sum_{v \in V} \left(\zvec[a_0, a_v] + \zvec[a_0,\bar a_v] \right)  \\
		&\hspace{2cm}+ \sum_{a \in \A_1 \setminus \{a_0\}} \sum_{ a' \in \A_2} \zvec[a, a'] \phi_{a_1}[a,a] u^i(a, a')\\
		& \ge \epsilon+ \left(\frac{\eta}{2}+\gamma\right)\sum_{v \in V} (\zvec[a_0,a_v] + \zvec[a_0,\bar a_v])+   \sum_{a \in \A_1 \setminus \{a_0\}} \sum_{ a' \in \A_2} \zvec[a, a'] \phi_{a_1}[a,a] u^i(a, a')\\
		& \ge u_1(z)+ \epsilon,
	\end{align*}
	where the first inequality comes from adding $\sum_{v \in V} \zvec[a_0,a_v]$ to both sides of Equation~\eqref{eq:balance}.
	Moreover, $\phi_{a_1}$ is feasible since for each constraint $c_{\bar v}$, $\bar  v \in V$, it has cost
	\begin{align*}
	&\sum_{v \in V} \left(\zvec[a_0,a_v] \phi_{a_1}[a_0,a_1] c_{\bar v}(a_1,a_v) + \zvec[a_0,\bar a_v] \phi_{a_1}[a_0,a_1] c_{\bar v}(a_1,a_v)\right) \\  
	&\hspace{2cm}+\sum_{a \in \A_1 \setminus \{a_0\}} \sum_{ a' \in \A_2} \zvec[a, a'] \phi_{a_1}[a,a] c_{\bar v}(a, a')\\
	&= \sum_{v \in V} \left(\zvec[a_0,a_v] \phi_{a_1}[a_0,a_1] c_{\bar v}(a_0,a_v) + \zvec[a_0,\bar a_v] \phi_{a_1}[a_0,a_1] c_{\bar v}(a_0,\bar a_v)\right) \\  
	&\hspace{2cm}+\sum_{a \in \A_1 \setminus \{a_0\}} \sum_{ a' \in \A_2}\zvec[a, a'] \phi_{a_1}[a,a] c_{\bar v}(a, a')\\
	&= c_{\bar v}(z)\le 0.
	 \end{align*}
	A similar argument shows that if $\sum_{v \in V} \zvec[a_0,a_v] < \sum_{v \in V} \zvec[a_0,\bar a_v]-\frac{2\epsilon}{\eta}$ then the deviation  $\phi_{a_2}$ is safe and increases the utility. 
	As a consequence of Equation~\eqref{eq:balance2}, it holds
	\begin{align}\label{eq:balance3}
		2\sum_{v \in V} \zvec[a_0,\bar a_v] \ge\sum_{v \in V} (\zvec[a_0, a_v]+\zvec[a_0,\bar a_v] ) -\frac{\epsilon}{\eta}= \sum_{a \in \A_2\setminus\{a_F\}} \zvec[a_0, a] -\frac{2\epsilon}{\eta},
	\end{align}
	where the first inequality comes from adding $\sum_{v \in V} \zvec[a_0,\bar a_v]$ to both sides of $\sum_{v \in V} \zvec[a_0,\bar a_v]|\ge \sum_{v \in V} \zvec[a_0,a_v]- \frac{2\epsilon}{\eta}$
	
	The next step is to show that it is if there is no safe deviation $\phi_{a_v}$, $v \in V$, that increases the utility, then there exists an independent set of size larger than $\ell^{\delta}$. 
	 Since $z$ is an Constrained $\epsilon$-Phi-equilibrium, for each $a_v$, $v\in V$ one of the following two conditions holds: i) $\phi_{a_v} \notin \Phi^\mcS_1(z)$ or ii) $u_1(\phi_{a_v}\diamond z)\le u_1(z) + \epsilon$.
	Let $V^1\subseteq V$ be the set of vertexes $v$ such that $\phi_{a_v}$ is not safe, \emph{i.e.}, $\phi_{a_v} \notin \Phi^\mcS_1(z)$,  and $V^2=V\setminus V^1$ be the set of $v$ such that $\phi_{a_v}$ does not increase the utility by more  than $\epsilon$ and are not in $V^1$, \emph{i.e.}, $u_1(\phi_{a_v}\diamond z)\le u_1(z)$ and $\phi_{a_v} \in \Phi_1^\mcS(z)$.
	We show that $|V^2|\le \ell-\ell^{1-\delta}$.
	Indeed, for each $v \in V^2$, deviation $\phi_{a_v}$ does not increase the utility and hence it holds:
	\begin{align*}
		\gamma \sum_{a \in \A_2 \setminus \{a_F\}} \zvec_[a_0,a]&  + \eta\frac{\ell-\ell^{1-\delta}}{\ell-\ell^{1-\delta}-1}   \sum_{v' \neq v}  \zvec[a_0,\bar a_{v'}]  +  \sum_{a \in A_1 \setminus \{a_0\}} \sum_{ a' \in \A_2} \zvec[a, a'] \phi_{a_1}[a,a] u^i(a, a')    \\
		&=\left(\sum_{v' \in V } \zvec[a_0,a] + \zvec[a_0,\bar a_v]\right) \phi[a_0,a_v] \gamma +\sum_{v' \neq v} \phi[a_0,a_v] \zvec[a_0,\bar a_{v'}]  \left(\gamma+\eta\frac{\ell-\ell^{1-\delta}}{\ell-\ell^{1-\delta}-1}  \right) \\ 
		&\hspace{2cm}+\sum_{a \in \A_1 \setminus \{a_0\}} \sum_{ a' \in \A_2} \zvec[a, a'] \phi_{a_1}[a,a] u^i(a, a') \\ &\le u_1(z) +\epsilon\\
		&  =\left(\gamma+ \frac{\eta}{2}\right) \sum_{a \in \A_2 \setminus \{a_F\}} \zvec[a_0,a] +  \sum_{a \in \A_1 \setminus \{a_0\}} \sum_{ a' \in \A_2} \zvec[a, a']  u^i(a, a')   +\epsilon,\\
	\end{align*}
	where the inequality holds since the lhs is the utility of the deviation $\phi_{a_v}$.
	
	This implies
	\[ 
	\left(\sum_{v' }  \zvec[a_0,\bar a_{v'}]-  \zvec[a_0,\bar a_{v}] \right)\eta\frac{\ell-\ell^{1-\delta}}{\ell-\ell^{1-\delta}-1} \le \frac{\eta}{2}  \sum_{a \in \A_2 \setminus \{a_F\}}  \zvec[a_0, a] +\epsilon \le \eta  \sum_{v \in V}  \zvec[a_0, \bar a_v] + 2\epsilon  ,
	\] 
	where the last inequality holds by Equation~\eqref{eq:balance3}.
	Hence, 
	\[     
	\zvec[a_0,\bar a_v] \frac{\ell-\ell^{1-\delta}}{\ell-\ell^{1-\delta}-1} \ge \left(\frac{\ell-\ell^{1-\delta}}{\ell-\ell^{1-\delta}-1}-1\right)\sum_{v' }  \zvec[a_0,\bar a_{v'}]  -2\epsilon/\eta,    
	\]
	and
	\begin{align}\label{eq:large}
		   \bar \zvec[a_0,a_v]  \ge \frac{1}{\ell-\ell^{1-\delta}} \sum_{v' }  \zvec[a_0,\bar a_{v'}] -2\epsilon/\eta .  
	\end{align}
	
	Suppose that $|V^2|>\ell-\ell^{1-\delta}$, and hence Equation~\eqref{eq:large} is satisfied by at least $|V^2|\ge \ell-\ell^{1-\delta}+1 $ vertexes.
	We need the following inequality. 
	\begin{align} \label{eq:contr}
		\frac{1}{\ell} \sum_{v' }  \zvec[a_0,\bar a_{v'}] &\ge \frac{1}{\ell} \sum_{a \in \A_2\setminus\{a_F\}} \zvec[a_0, a] -\frac{2\epsilon}{\ell\eta}
		\ge \frac{\alpha}{4\ell}-\frac{2\epsilon}{\ell\eta}
		= \frac{\alpha}{4\ell}-\frac{\alpha}{8\ell^3} 
		\ge  \frac{\alpha}{8\ell} 
		=\frac{2\ell}{\eta} \left(\frac{\alpha^2}{16\ell^2 }  \right)
			=\frac{2\ell}{\eta} \epsilon 
	\end{align}
	where the first inequality comes from Equation~\eqref{eq:balance3}, and the second one by Equation~\eqref{eq:highProb}.
	Then, summing over the $|V^2|$ inequalities we get
	\begin{align*}
		\sum_{v \in V^2} \bar \zvec[a_0,a_v]&\ge  (\ell-\ell^{1-\delta}+1 ) \left(\frac{1}{\ell-\ell^{1-\delta}} \sum_{v' }  \zvec[a_0,\bar a_{v'}] -2\epsilon/\eta\right) \\
		& \ge \sum_{v' }  \zvec[a_0,\bar a_{v'}] + \frac{1}{\ell} \sum_{v' } \zvec[a_0,\bar a_{v'}]  -2\ell \frac{\epsilon}{\eta}\\
		&> \sum_{v' }  \zvec[a_0,\bar a_{v'}],
	\end{align*}
	where the last inequality follows from equation~\eqref{eq:contr}.
	 Hence, we reach a contradiction and $|V^2|\le \ell-\ell^{1-\delta}$.
	
	
	To conclude the proof, we show that $V^1$ is an independent set. Since $|V^1|\ge |V|-|V^2|=\ell^{1-\delta}$ we reach a contradiction.
	Let $v$ and $v'$ be two nodes in $V^1$ and w.l.o.g. let $\zvec[a_0,a_v]\ge \zvec[a_0,a_{v'}]$. We show that $(v,v')\notin E$. Since $v'\in V^1$, $\phi_{a_v}$ is not a safe deviation for player $1$ with respect to constraint $c^{v'}$. if $(v,v')\in E$, then
	\begin{align*}
	 \sum_{a^1 \in \A_1,a^2\in \A_2} \sum_{a \in\ \A_1} &\phi[a^1,a] \zvec[a^1,a^2] c_v(a,a^2) \\
	 &= \zvec[a_0,a_v']- \sum_{v'': (v'',v')\in E} \zvec[a_0,a_{v''}] -\frac{1}{4\ell} \zvec[a_0,a_F] c_v(a,a^2)\\
	 &\hspace{2cm}+  \sum_{a^1 \in \A_1 \setminus \{a_0\},a^2\in A_2} \sum_{a \in \A_1} \phi[a^1,a] \zvec[a^1,a^2] c_v(a,a^2)  \\
	  & \le \zvec[a_0,a_v'] -  \zvec[a_0,a_{v}] -\frac{1}{4\ell} \zvec[a_0,a_F] c_v(a,a^2)+  \\
	  & \hspace{2cm}+\sum_{a^1 \in \A_1 \setminus \{a_0\},a^2\in \A_2} \sum_{a \in \A_1} \phi[a^1,a] \zvec[a^1,a^2] c_v(a,a^2)\\
	  & \le -\frac{1}{4\ell} \zvec[a_0,a_F] c_v(a,a^2)+  \sum_{a^1 \in \A_1 \setminus \{a_0\},a^2\in \A_2} \sum_{a \in \A_1} \phi[a^1,a] \zvec[a^1,a^2] c_v(a,a^2)\\
	  & = c_v(z)\le 0.
	\end{align*}
	 Hence, $(v,v')\notin E$.
	 Since $V^1$ is an independent set of size at least $\ell^{1-\delta}$ we reach a contradiction. This concludes the proof.
\end{proof}
