# Supplementary material for: Multi-Agent Contract Design: How to Commission Multiple Agents with Individual Outcome
Source: arXiv:2301.13654 source file (2023-01-31)
Supplement: Supplementary file 8 [file appendixOptimal.tex]

\section{Proofs Omitted from Section~\ref{sec:optimal} }\label{sec:app_optimal}


\minmax*

\begin{proof}
	First, it is easy to see that
	%
	\begin{align*}
		\sup_{\phi_i \in \Phi_i^\mcS(\zvec)} u_i(\phi_i \diamond \zvec)=
		\sup_{\phi_i\in\Phi_i} \inf_{\etavec_i \in \mathbb{R}^{m}_+} &\left(u_i(\phi_i \diamond \zvec)-\etavec_i^{\top} \cvec_i(\phi_i \diamond \zvec)\right).
	\end{align*}
	%
	Indeed, for every $\phi_i \notin  \Phi_i^\mcS(\zvec)$, it holds that the vector $\cvec_i(\phi_i\diamond \zvec)$ has at least one positive component, and, thus, the vector of Lagrange multipliers $\etavec_i$ can be selected so that $u_i(\phi_i \diamond \zvec)-\etavec_i^{\top} \cvec_i(\phi_i \diamond \zvec)$ goes to $-\infty$.
	%
	This implies that the supremum over $\Phi_i$ cannot be attained in $\Phi_i^\mcS(\zvec)$.
	%å
	On the other hand, for every $\phi_i \in  \Phi_i^\mcS(\zvec)$, all the components of $\cvec_i(\phi_i\diamond \zvec)$ are negative, and, thus, the $\inf$ is achieved by $\etavec_i=\zerovec$.
	%
	This proves the first equality.
	
	Then, the second equality directly follows from the generalization of the max-min theorem for unbounded domains (see~\citep[Proposition~2.3]{ekeland1999convex}), which allows us to swap the $\sup$ and the $\inf$.
	%
\end{proof}

\begin{lemma}\label{lem:lemmaa1}
	For any two real-valued functions $f(x)$ and $g(x)$ with $g(x)\le c$ then $\min(f(x), g(x))\le\min(f(x), c)$.
\end{lemma}

\begin{proof}
	We can identify three sets $I_1, I_2$ and $I_3$ defined as follows:
	\begin{align*}
		I_1&\coloneqq\{x\, s.t.\, f(x)\ge c\}\\
		I_2&\coloneqq\{x\, s.t.\, g(x)\le f(x)\le c\}\\
		I_3&\coloneqq\{x\, s.t.\, f(x)\le g(x)\le c\}.
	\end{align*}
	Then for all $x\in I_1$ we have that
	\(
	\min(f(x), c)=c\ge\min(f(x), g(x))=g(x),
	\)
	while for all $x\in I_2$ we have that
	\(
	\min(f(x), c)=f(x)\ge\min(f(x), g(x))=g(x).
	\)
	Finally for all $x\in I_3$ we have
	\(
	\min(f(x), c)=f(x)=\min(f(x), g(x))=f(x).
	\)
	In all three sets we have that $\min(f(x), c)\ge\min(f(x), g(x))$.
\end{proof}

\begin{lemma}\label{lem:lemmaa2}
	For all $\etavec_i\in\D^c$ it holds that
	\[
	\sup\limits_{\phi_i\in\Phi_i}\left(u_i(\phi_i\diamond\zvec)-\etavec_i^\top\cvec_i(\phi_i\diamond\zvec)\right)\ge 1
	\]
\end{lemma}

\begin{proof}
	Thanks to Assumption~\ref{ass:strictly} we have that for all $\zvec\in\Delta(\A)$ we have that there exists $\tilde\phi_i\in\Phi_i^\mcS(\zvec)$ such that $\cvec_i(\tilde\phi_i\diamond\zvec)\preceq-\rho\onevec$. Then, for all $\etavec_i\in\D^c$ we have:
	\[
	\etavec_i^\top \cvec_i(\tilde\phi_i\diamond \zvec)\le -\rho\|\etavec_i\|_1\le -1.
	\]
	This easily concludes the proof of the statement
	\[
	\sup\limits_{\phi_i\in\Phi_i}\left(u_i(\phi_i\diamond\zvec)-\etavec_i^\top\cvec_i(\phi_i\diamond\zvec)\right)\ge u_i(\tilde\phi_i\diamond\zvec)-\etavec_i^\top\cvec_i(\tilde\phi_i\diamond\zvec)\ge 1,
	\]
	as $u_i$ is positive.
\end{proof}

\begin{lemma}\label{lem:lemmaa3}
	For all $\etavec_i\in\D$ we have
	\[
	\inf\limits_{\etavec_i\in\D}\sup\limits_{\phi_i\in\Phi_i}\left(u_i(\phi_i\diamond\zvec)-\etavec_i^\top\cvec_i(\phi_i\diamond\zvec)\right)\le 1
	\]
\end{lemma}

\begin{proof}
	Since $u_i\le 1$ we have that
	\[
	\inf\limits_{\etavec_i\in\D}\sup\limits_{\phi_i\in\Phi_i}\left(u_i(\phi_i\diamond\zvec)-\etavec_i^\top\cvec_i(\phi_i\diamond\zvec)\right)\le 1-\sup\limits_{\etavec_i\in\D}\inf\limits_{\phi_i\in\Phi_i} \etavec_i^\top\cvec_i(\phi_i\diamond \zvec).
	\]
	Next we claim that $\sup\limits_{\etavec_i\in\D}\inf\limits_{\phi_i\in\Phi_i} \etavec_i^\top\cvec_i(\phi_i\diamond \zvec)\ge 0$. This follows from the fact that for all negative components of $\cvec_i(\phi_i\diamond \zvec)$ then the corresponding components of $\etavec_i$ will be $0$. This concludes the statement.
\end{proof}



\duality*

\begin{proof}
	In Lemma~\ref{lem:minmax} we already showed that:
	\begin{align*}
		\sup_{\phi_i \in \Phi_i^\mcS(\zvec)} u_i(\phi_i \diamond \zvec)&=
		\sup\limits_{\phi_i\in\Phi_i} \inf_{\etavec_i \in \mathbb{R}^{m}_+} \left(u_i(\phi_i\diamond \zvec)-\etavec_i^{\top} \cvec_i(\phi_i \diamond z)\right) \\
		&=\inf_{\etavec_i \in \mathbb{R}^{m}_+}  \sup\limits_{\phi_i\in\Phi_i}\left(u_i(\phi_i \diamond\zvec)-\etavec_i^{\top} \cvec_i(\phi_i \diamond\zvec)\right).
	\end{align*}
	Note that to prove the statement it is enough to prove that:
	\[
	\inf_{\etavec_i \in \mathbb{R}^{m}_+}  \sup\limits_{\phi_i\in\Phi_i}\left(u_i(\phi_i \diamond\zvec)-\etavec_i^{\top} \cvec_i(\phi_i \diamond\zvec)\right)=\inf_{\etavec_i \in\D}  \sup\limits_{\phi_i\in\Phi_i}\left(u_i(\phi_i \diamond\zvec)-\etavec_i^{\top} \cvec_i(\phi_i \diamond\zvec)\right)
	\]
	and more specifically that:
	\[
	\inf_{\etavec_i \in \mathbb{R}^{m}_+}  \sup\limits_{\phi_i\in\Phi_i}\left(u_i(\phi_i \diamond\zvec)-\etavec_i^{\top} \cvec_i(\phi_i \diamond\zvec)\right)\ge\inf_{\etavec_i \in\D}  \sup\limits_{\phi_i\in\Phi_i}\left(u_i(\phi_i \diamond\zvec)-\etavec_i^{\top} \cvec_i(\phi_i \diamond\zvec)\right)
	\]
	since the reverse inequality holds trivially.
	We can show this by the following inequalities:
	\begin{align*}
		\inf_{\etavec_i \in \mathbb{R}^{m}_+}  &\sup\limits_{\phi_i\in\Phi_i}\left(u_i(\phi_i \diamond\zvec)-\etavec_i^{\top} \cvec_i(\phi_i \diamond\zvec)\right)\\
		&=\min\left(\inf_{\etavec_i \in\D}  \sup\limits_{\phi_i\in\Phi_i}\left(u_i(\phi_i \diamond\zvec)-\etavec_i^{\top} \cvec_i(\phi_i \diamond\zvec)\right), \inf_{\etavec_i \in \D^c}  \sup\limits_{\phi_i\in\Phi_i}\left(u_i(\phi_i \diamond\zvec)-\etavec_i^{\top} \cvec_i(\phi_i \diamond\zvec)\right)\right)\\
		&\ge\min\left(\inf_{\etavec_i \in\D}  \sup\limits_{\phi_i\in\Phi_i}\left(u_i(\phi_i \diamond\zvec)-\etavec_i^{\top} \cvec_i(\phi_i \diamond\zvec)\right), 1\right)\\
		&=\inf_{\etavec_i \in\D}  \sup\limits_{\phi_i\in\Phi_i}\left(u_i(\phi_i \diamond\zvec)-\etavec_i^{\top} \cvec_i(\phi_i \diamond\zvec)\right),
	\end{align*}
	where the first inequality hold thanks to Lemma~\ref{lem:lemmaa1} and Lemma~\ref{lem:lemmaa2}, while that last equation follows from Lemma~\ref{lem:lemmaa3}. 
\end{proof}

\deltaOPTProblem*

\begin{proof}
	By definition we have that:
	$L_{\bar\D,\epsilon} =\ell(\tilde\zvec^\star)$, where $\tilde\zvec^\star$ is a solution to the problem
	\[
	\textnormal{P1}\coloneqq
	\begin{cases}
		\tilde\zvec^\star\in\arg\max\limits_{\zvec\in\mcS} &\ell(\zvec)\, s.t.\\
		&\epsilon+u_i(\tilde\zvec^\star)\ge\max\limits_{\phi_i\in\Phi_i}\left(u_i(\phi_i\diamond\tilde\zvec^\star)-\tilde\etavec_i^{\star,\top}\cvec_i(\phi_i\diamond\tilde\zvec^\star)\right)\\
		&\tilde\etavec_i^\star\in\arg\inf\limits_{\etavec_i\in\bar\D}\sup\limits_{\phi_i\in\Phi_i}\left(u_i(\phi_i\diamond\tilde\zvec^\star)-\etavec_i^{\top}\cvec_i(\phi_i\diamond\tilde\zvec^\star)\right)
	\end{cases}
	\]
	
	On the other hand, call $\zvec^\star$ the optimal Constrained Phi-equilibrium. This is a solution to the problem:
	\[
	\textnormal{P2}\coloneqq
	\begin{cases}
		\zvec^\star\in\arg\max\limits_{\zvec\in\mcS} &\ell(\zvec)\, s.t.\\
		&u_i(\zvec^\star)\ge\max\limits_{\phi_i\in\Phi_i}\left(u_i(\phi_i\diamond\zvec^\star)-\etavec_i^{\star,\top}\cvec_i(\phi_i\diamond\zvec^\star)\right)\\
		&\etavec_i^\star\in\arg\inf\limits_{\etavec_i\in\D}\sup\limits_{\phi_i\in\Phi_i}\left(u_i(\phi_i\diamond\zvec^\star)-\etavec_i^{\top}\cvec_i(\phi_i\diamond\zvec^\star)\right)
	\end{cases}
	\]
	which has value $L_{\D,0}=\ell(\zvec^\star)$.
	
	Moreover, thanks to Lemma~\ref{lem:duality} and since $\bar\D$ is $\delta$-optimal we have that:
	\[
	\max\limits_{\phi_i\in\Phi_i}\left(u_i(\phi_i\diamond\tilde\zvec^\star)-\tilde\etavec_i^{\star,\top}\cvec_i(\phi_i\diamond\tilde\zvec^\star)\right)\le\max\limits_{\phi_i\in\Phi_i}\left(u_i(\phi_i\diamond\zvec^\star)-\etavec_i^{\star,\top}\cvec_i(\phi_i\diamond\zvec^\star)\right)+\delta
	\]
	which implies that feasible correlated strategies of problem P2 are feasible  correlated strategies of problem P1, and thus problem P1 as long as $\delta\ge \epsilon$. Thus problem P1 is the problem of maximizing the same objective function over a larger set then problem P2 and thus $L_{\bar\D,\epsilon}\ge L_{\D,0}$.
\end{proof}


%\begin{proof}
%	As a first step, we show that 
%	
%	\begin{align}\label{eq:bounded}
	%		&\inf_{ \etavec_i \in \D}\,\sup_{\phi_i\in\Phi_i } \left(u_i(\phi_i \diamond \zvec)-\etavec_i^\top\cvec_i(\phi_i\diamond \zvec)\right)\le\inf_{ \etavec_i \in\Reals_+^{m}}\,\sup_{\phi_i\in\Phi_i } \left(u_i(\phi_i\diamond \zvec)-\etavec_i^\top \cvec_i(\phi^i \diamond \zvec)\right).
	%	\end{align}
%	
%	To do so, notice that for any $\etavec_i\notin\D$, we have 
%	\[
%	\sup_{\phi_i \in\Phi_i}\left(u_i(\phi_i\diamond \zvec)-\etavec_i^\top \cvec_i(\phi_i\diamond \zvec)\right)\ge 1
%	\]
%	The previous inequality follows from observing that, thank to Assumption~\ref{ass:strictly}, there exists $\phi_i$ such that $\cvec_i(\phi_i\diamond \zvec)\le -\rho\onevec$ and thus $\etavec_i^\top\cvec_i(\phi_i\diamond\zvec)\le-\rho\|\etavec_i\|_1\le-1$ where the last inequality follows from the fact that $\etavec_i\notin\D$.
%	Moreover we also have
%	\[
%	1\ge \inf_{\etavec_i\in\Reals_+^{m}}\,\sup_{\phi^i\in\Phi_i} \left(u_i(\phi_i\diamond \zvec)-\etavec_i^\top \cvec_i(\phi^i \diamond \zvec)\right),
%	\]
%	where the first inequality holds because by Assumption~\ref{ass:strictly}, there exists a deviation $\phi^i$ that provides value at least $\langle\eta',\rho \textbf{1} \rangle > 1$.
%	%
%	Then, we have:
%	%\begin{subequations}
%	\begin{align*}
	%		\sup_{\phi^i}\,\inf_{\eta\in\D} \left(U^i(\phi^i z)-\eta^i C(\phi^i z)\right) &\ge \sup_{\phi^i }\,\inf_{\eta\ge 0} \left(U^i(\phi^i z)-\eta^i C(\phi^i z)\right)\\
	%		& =V_{z,i}\\
	%		&=\inf_{\eta\ge 0}\,\sup_{\phi^i} \left(U^i(\phi^i z)-\eta^i C(\phi^i z)\right)\\
	%		&\ge \inf_{ \eta\in\D}\,\sup_{\phi^i} \left(U^i(\phi^i z)-\eta^i C(\phi^i z)\right),
	%	\end{align*}
%	%\end{subequations}
%	where the first inequality holds since on the lefthand side we have a more restrictive set of dual variables, the equalities hold by strong duality, and the last inequality holds by Eq.~\eqref{eq:bounded}.
%	%
%	Finally, by the  max–min inequality 
%	\[
%	\sup_{\phi^i }\,\inf_{\eta\in\D} \left(U^i(\phi^i z)-\eta^i C(\phi^i z)\right)\le \inf_{\eta\in\D}\,\sup_{\phi^i } \left(U^i(\phi^i z)-\eta^i C(\phi^i z)\right).
%	\] 
%	This proves our statement.
%\end{proof}


\gridisemopt*
\begin{proof}
	By Lemma \ref{lem:duality}, we know that for each player there exists an $\etavec_i^\star\in\D$ such that $\max_{\phi \in \Phi_i^\mcS(\zvec)} u_i(\phi_i\diamond \zvec)= \max\limits_{\phi_i\in\Phi_i}\left(u_i(\phi_i\diamond \zvec)-\etavec_i^{\star,\top} \cvec_i(\phi_i\diamond \zvec)\right)$.
	By construction of $\D_\epsilon$ there exists a $\bar \etavec_i \in \D_\epsilon $ such that $||\bar \etavec_i-\etavec_i^\star||_\infty \le \epsilon$.
	Thus
	\begin{align*}
		\max_{\phi \in \Phi_i^\mcS(\zvec)} u_i(\phi_i\diamond \zvec)&= \max\limits_{\phi_i\in\Phi_i}\left(u_i(\phi_i\diamond \zvec)-\etavec_i^{\star,\top} \cvec_i(\phi_i\diamond \zvec)\right)\\
		&\le \max\limits_{\phi_i\in\Phi_i}\left(u_i(\phi_i\diamond \zvec)-\bar \etavec_i^\top \cvec_i(\phi_i\diamond \zvec)\right)+ m \epsilon,
	\end{align*}
	where the last inequality comes the fact that:
	%
	\[
	|(\etavec_i^\star-\bar\etavec_i)^\top\cvec_i(\phi_i\diamond\zvec)|\le \|\cvec_i(\phi_i\diamond\zvec)\|_1\|\etavec_i^\star-\bar\etavec_i\|_\infty\le m\epsilon
	\]
	%
	as $\cvec_i\in [-1,1]^{m}$.
\end{proof}



\uniform*
\begin{proof}
	The proof exploits a probability interpretation of the Lagrange multipliers. Let $\etavec^\star$ be the optimal multipliers, \ie, $\etavec^\star\in\argmin_{\etavec\in\D}\max_{\phi_i\in\Phi_i}\left(u_i(\phi_i\diamond \zvec)-\etavec^{\top} \cvec_i(\phi_i\diamond \zvec)\right)$. Now consider a basis $\Gamma=\{\frac{1}{\rho}\evec_j\}_{j\in [m]}\cup\{\zerovec\}$ for $\D$.
	By Carathoedory's theorem there exists a distribution $\gamma\in\Delta(\Gamma)$ such that $\etavec^\star=\sum_{\etavec\in\Gamma}\gamma_{\etavec}\etavec$. Assume that $\epsilon$ and $\rho$ are such that $\sfrac{1}{\epsilon\rho}$ is an integer and take $\sfrac{1}{\rho\epsilon}$ samples from the distribution $\gamma$ and call $\tilde\etavec$ the resulting empirical mean.
	
	First, we argue that $\tilde\etavec\in\D_\epsilon$. Indeed $\tilde\etavec_j=\frac{k_j}{\sfrac{1}{\rho\epsilon}}\frac{1}{\rho}=\epsilon\left(\frac{k_j}{\sfrac{1}{\rho\epsilon}}\frac{1}{\rho\epsilon}\right)=\epsilon k_j$ where $k_j\in\mathbb{N}$ and thus we have that $\tilde\etavec\in\D_\epsilon$.\footnote{If $\epsilon$ if not such that $\sfrac{1}{\rho\epsilon}\in\mathbb{N}$ then the one can take $\lceil\sfrac{1}{\rho\epsilon}\rceil$ samples from $\gamma\in\Delta(\Gamma)$ and then the statement hold for a slightly smaller $\epsilon^\prime<\epsilon$ defined as $\epsilon^\prime:=\frac{1}{\lceil\sfrac{1}{\rho\epsilon}\rceil}\frac{1}{\rho}$.}
	
	Now we show that with high probability $\tilde\etavec\in\D_\epsilon$ is close (in terms of utilities) to the optimal multiplier $\etavec^\star$.
	First observe that:
	\begin{subequations}\label{eq:inequalitylemmaProbs}
	\begin{align}
	\etavec_i^{\star,\top}\cvec_i(\phi_i\diamond\zvec)&:=\sum\limits_{a_i\in\A^i,b_{i}\in\A^{i}}\left(\phi_i[b,a_i]\sum\limits_{\avec_{-i}\in\A^{-i}}\etavec^{\star,\top}\cvec_i(a_i,\avec_{-i})\zvec[b,\avec_{-i}]\right)\\
	&\le\sum\limits_{a_i\in\A^i,b_{i}\in\A^{i}}\left(\phi_i[b,a_i]\left(\delta_{a_i,b}+\sum\limits_{\avec_{-i}\in\A^{-i}}\tilde\etavec^{\top}\cvec_i(a_i,\avec_{-i})\zvec[b,\avec_{-i}]\right)\right)\\
	&=\sum\limits_{a_i\in\A^i,b_{i}\in\A^{i}}\left(\phi_i[b,a_i]\sum\limits_{\avec_{-i}\in\A^{-i}}\tilde\etavec^{\top}\cvec_i(a_i,\avec_{-i})\zvec[b,\avec_{-i}]\right)+\sum\limits_{a_i\in\A^i,b_{i}\in\A^{i}}\phi_i[b,a_i]\delta_{a_i,b}\\
	&=\tilde\etavec_i^{\top}\cvec_i(\phi_i\diamond\zvec)+\sum\limits_{a_i\in\A^i,b_{i}\in\A^{i}}\phi_i[b,a_i]\delta_{a_i,b}
	\end{align}
	\end{subequations}
	where the inequality comes from applying the Hoeffeding's inequality to every $a_i,b\in\A_i$:
	\[
	\left|\sum\limits_{a_{-i}\in\A^{-i}}\left(\tilde\etavec-\etavec^{\star}\right)^\top\cvec_i(a_i,a_{-i})\zvec[b,\avec_{-i}]\right|\le \delta_{a_i,b}
	\]
	where $\delta_{a_i,b}=\frac{2}{\rho}\sqrt{\frac{2}{\sfrac{1}{\rho\epsilon}}\log\left(\frac{2}{p_{a_i,b}}\right)}\left(\sum\limits_{\avec_{-i}\in\A^{-i}}\zvec[b,\avec_{-i}]\right)$ since the range of the each sample is $\frac{1}{\rho}\left(\sum_{\avec_{-i}\in\A^{-i}}\zvec[b,\avec_{-i}]\right)$.
	
	Moreover, for Hoeffeding's inequality, for every $a_i,b\in\A^i$ the above inequality holds with probability at least $1-p_{a_i,b}$ and thus holds for all the $a_i,b\in\A^i$ simultaneously, with probability at least $p:=\sum_{a_i,b\in\A^i}p_{a_i,b}$.
	%
	If then we take $p_{a_i, b}:=\frac{1}{2|\A^i|^2}$ for all $a_i,b\in\A^i$, then we have that $p=1/2>0$ and $\delta:=\delta_{a_i,b}=\frac{2}{\rho}\sqrt{\frac{2}{\sfrac{1}{\rho\epsilon}}\log\left(|\A^i|\right)}\left(\sum\limits_{\avec_{-i}\in\A^{-i}}\zvec[b,\avec_{-i}]\right)$
	
	%
	Now the following holds with probability at lest $1/2$:
	\[
	\left|\sum\limits_{a_{-i}\in\A^{-i}}\left(\tilde\etavec-\etavec^{\star}\right)^\top\cvec_i(a_i,a_{-i})\zvec[b,\avec_{-i}]\right|\le \delta\left(\sum_{\avec_{-i}\in\A^{-i}}\zvec[b,\avec_{-i}]\right),\quad\forall a_i,b\in\A^i
	\]
	
	The proof is concluded by observing plugging this definition of $\delta=\delta_{a_i,b}$ in Equation~\eqref{eq:inequalitylemmaProbs} yields
	\(
	\sum_{a_i\in\A^i,b_{i}\in\A^{i}}\phi_i[b,a_i]\delta_{a_i,b}=\delta,
	\)
	and we can conclude that:
	\[
	\etavec_i^{\star,\top}\cvec_i(\phi_i\diamond\zvec)\le\tilde\etavec_i^{\top}\cvec_i(\phi_i\diamond\zvec)+\delta.
	\]
	This holds with positive probability, and thus shows the existence of such $\tilde\etavec\in\D_\epsilon$ for which the above inequality holds and thus $\D_\epsilon$ is $\left(2\sqrt{\frac{2\epsilon}{\rho}\log(|\A^i|)}\right)$-optimal.
\end{proof}

%OLD
%\begin{proof}
%	
%
%	The proof exploits a probability interpretation of the Lagrangian multipliers.
%	Let $\etavec^*$ be an optimal lagrangian multiplier, \emph{i.e.}, $\etavec^* \in \argmin_{\etavec \in \D} \max_{\phi \in \Phi^i}\left(u_i(\phi_i\diamond \zvec)-\etavec^{\top} \cvec_i(\phi_i\diamond \zvec)\right) $. Let $\Gamma=\{\frac{1}{\rho}\mathbf{1}_j\}_{j \in m } \cup \textbf{0}$, where $\mathbf{1}_j \in \D$ is the vector in which the $j$ component is one and all the other components are $0$ while $\textbf{0}$ is the $m$-dimentional $0$ vector.
%	Then, by Caratheodory theorem there exists a distribution $\gamma \in \Delta_{\Gamma}$ such that $\etavec^*=\sum_{\etavec \in \Gamma} \gamma_{\eta} \eta$.
%	Let $\tilde \etavec$ be the empirical mean of $\frac{1}{\rho\epsilon}$  i.i.d. samples drawn from the distribution $\gamma$.
%	It is easy to see that $\tilde \etavec$ belong to $\D_{\epsilon}$ with probability $1$.
%	Now, we show that $\tilde \etavec$ with probability strictly greater than $0$ satisfies  all the constraints:
%	\begin{align}\label{eq:deviation}
%	\sum_{\avec:z_i=a} z[\avec] [u^i(a',\avec_{-i})-\tilde \etavec c^i(a',a_{-i})] \le \sum_{\avec:z_i=a} z[\avec] [u^i(a',\avec_{-i})- \etavec^* c^i(a',a_{-i})] +\delta \sum_{\avec:z_i=a} z[\avec]\quad  \forall a,a' \in \A^i.
%	\end{align}
%	In particular,
%	given an $a,a' \in \A^i$, by Hoeffding bound to the random variable $\tilde \etavec c^i(a',a_{-i})$, Equation~\eqref{eq:deviation} holds with probability at least $1-e^{-\frac{2\delta^2/(\rho\epsilon)}{4 \rho^2}}=1-e^{-\frac{\delta^2}{2\epsilon}}$.
%	Applying the union bound over all the couples $a,a'\in \A^i$, we get that all the Equations~\eqref{eq:deviation} hold simultaneously with probability at least $1-|\A^i| e^{-\frac{\delta^2}{2\epsilon}}$.
%	Then, for $\delta=2\sqrt{\epsilon\log(|\A^i|)}$ there exists a $\bar \etavec \in \D_{\epsilon}$ that satisfies all the inequalities.
%	
%	We show that this approximation can be extended to all the deviations $\phi \in \Phi^i$. Let $\phi \in \Phi^i$ be any deviation, then
%		\begin{align*}
%	 u_i(\phi_i\diamond \zvec)-\etavec_i^{\star,\top} \cvec_i(\phi_i\diamond \zvec)&= \sum_{a ,a'\in \A^i} \phi[a,a'] \sum_{\avec:z_i=a} z[\avec] [u^i(a',\avec_{-i})- \etavec^{*,\top} c^i(a',a_{-i})] \\
%	 & \le  \sum_{a ,a'\in \A^i} \phi[a,a'] [ \sum_{\avec:z_i=a} z[\avec] [u^i(a',\avec_{-i})- \bar\etavec^{\top} c^i(a',a_{-i})+\delta]\\
%	 & = \sum_{a ,a' \in \A^i} \phi[a,a'] [ \sum_{\avec:z_i=a} z[\avec] [u^i(a',\avec_{-i})- \bar\etavec^{\top} c^i(a',a_{-i})]+ \sum_{a ,a' \in \A^i} \phi[a,a'] \sum_{\avec:z_i=a} z[\avec] \delta\\
%	 &= \sum_{a ,a' \in \A^i} \phi[a,a'] [ \sum_{\avec:z_i=a} z[\avec] [u^i(a',\avec_{-i})- \bar\etavec^{\top} c^i(a',a_{-i})]+ \delta\\
%	 & = u_i(\phi_i\diamond \zvec)-\bar \etavec_i^{\top} \cvec_i(\phi_i\diamond \zvec) + \delta.
%	\end{align*}
%	
%	Then,
%	\begin{align*}
%	\max_{\phi \in \Phi_i^\mcS(\zvec)} u_i(\phi_i\diamond \zvec) &= \max\limits_{\phi_i\in\Phi_i}\left(u_i(\phi_i\diamond \zvec)-\etavec^{\star,\top} \cvec_i(\phi_i\diamond \zvec)\right)\\
%	&\le \max\limits_{\phi_i\in\Phi_i}\left(u_i(\phi_i\diamond \zvec)-\bar \etavec_i^\top \cvec_i(\phi_i\diamond \zvec)\right)+ \delta,
%	\end{align*}
%	where the first equality comes from Lemma~\ref{lem:duality}.
%	This concludes the proof.
%	
%\end{proof}
