# Supplementary material for: Multi-Agent Contract Design: How to Commission Multiple Agents with Individual Outcome
Source: arXiv:2301.13654 source file (2023-01-31)
Supplement: Supplementary file 9 [file appendixPrelim.tex]

\section{On the Weaknesses of the Guarantees of the Algorithm of~\citet{chenfinding}}\label{app:weakness}
The Algorithm of~\citet{chenfinding} finds a distribution $\mu$ over correlated strategies  $\Delta_{\A}$ such that:
\begin{equation}\label{eq:expectation_IC}
\mathbb{E}_{\zvec\sim\mu}\left[\max\limits_{\phi_i\in\Phi_i^\mcS(\zvec)}u_i(\phi_i\diamond\zvec)-u_i(\zvec)\right]\le 0.
\end{equation}
However, here we claim that this solution concept inherits some weaknesses from the non-convexity of the equilibria set that we proved in Theorem~\ref{thm:convex}.
Indeed, consider the same instance of Theorem~\ref{thm:convex} and consider the uniform distribution $\mu$ over $\{\zvec_1, \zvec_2\}$. In Theorem~\ref{thm:convex} we proved that $\max_{\phi_i\in\Phi_i^\mcS(\zvec^1)}u_i(\phi_i\diamond\zvec^1)-u_i(\zvec^1)\le 0$ for all $i\in\{1,2\}$ and $\max_{\phi_i\in\Phi_i^\mcS(\zvec^2)}u_i(\phi_i\diamond\zvec^2)-u_i(\zvec^2)\le 0$ for all $i\in\{1,2\}$ and thus Equation~\eqref{eq:expectation_IC} holds over the distribution $\mu$.

However we show that the expected correlated strategy $\zvec^3$ derived from distribution $\mu$, \ie $\zvec^3=\mathbb{E}_{\zvec\sim\mu}[\zvec]=\frac{1}{2}\zvec^1+\frac{1}{2}\zvec^2$, it is not a feasible equilibrium, or an approximate one.

Indeed, in Theorem~\ref{thm:convex}, we proved that $\max_{\phi_2\in\Phi_2^\mcS(\zvec^3)}u_2(\phi_2\diamond\zvec^3)-u_2(\zvec^3)\ge\frac{1}{3}$, showing that the average correlated strategies returned by their Algorithm is not an equilibrium nor close to it.

This comes from the peculiar fact about Constrained Phi-equilibria that exhibit non-convex set of solutions, which is in striking contrast with the unconstrained case.
Indeed the guarantees of Equilibria~\eqref{eq:expectation_IC} would imply that $\mathbb{E}_{\zvec\sim\mu}[\zvec]$ is a equilibrium in the unconstrained case in which the set of equilibria is convex.



\section{Proofs Omitted from Section~\ref{sec:prelim} }

\existence*
\begin{proof}
	With assumption~\ref{ass:strictly} \citet[Theorem~2.1]{altman2000constrained} proves the existence of a constrained Nash equilibrium. In our setting this is equivalent to a product distribution $\zvec=\otimes_{i\in[N]}\xvec_i$ so that it is a Constrained Phi-equilibrium for any set of deviations $\Phi_i$.\footnote{As common in the normal form game literature, for any distribution $\xvec\in\Delta(X)$ and $\yvec\in\Delta(Y)$, $\xvec\otimes\yvec\in\Delta(X\times Y)$ is the product distribution defined as $(\xvec\otimes\yvec)[a,b]=\xvec[a]\yvec[b]$ for $a\in X$ and $b\in Y$.}
	This is easily seen by observing that a Constrained Nash Equilibria is defined as:
	\[
	\sum\limits_{\avec\in\A}u_i\left(\prod_{j\in[N]}\xvec_j(a_j)\right)\ge 	\sum\limits_{\avec\in\A}u_i\left(\tilde\xvec_i(a_j)\prod_{j\in[N]\setminus \{i\}}\xvec_i(a_i)\right)
	\]
	for all $\tilde\xvec_i\in\Delta(\A^i)$ s.t. $\xvec_i\otimes\xvec_{-i}\in\mcS$.
	
	On the other hand it easily seen that for all $\phi_i\in\Phi_i(\zvec)$ there exists some $\tilde\xvec_i\in\Delta(\A^i)$ such that 
	\[
	\phi_i\diamond\left( \otimes_{j\in[N]}\xvec_{j}\right) = \tilde\xvec_i\otimes\xvec_{-i}
	\]
	and $\tilde\xvec_i\otimes\xvec_{-i}\in\mcS$.
	
	This is proved by the following calculations:
	\begin{align}
		\phi_i\diamond\left( \otimes_{j\in[N]}\xvec_{j}\right)[a_i,\avec_{-i}]&:=\sum\limits_{b\in\A^i}\phi_i[b,a_i]\xvec_i(b)\xvec_{-i}(\avec_{-i})\\
		&=\tilde\xvec_i(a_i)\otimes\xvec_{-i}(\avec_{-i}),
	\end{align}
	where $\tilde\xvec_i(a_i):=\sum_{b\in\A^i}\phi_i[b,a_i]\xvec_i(b)$ and $\tilde\xvec_i\in\Delta(A^i)$ since, by definition, $\sum_{a_i\in\A^i}\phi_i[b,a_i]=1$ for all $b\in\A^i$.
	
	This proves that a Constrained Nash Equilibrium is a Phi-Constrained Equilibrium for all $\Phi$. 
\end{proof}
