# Supplementary material for: Multi-Agent Contract Design: How to Commission Multiple Agents with Individual Outcome
Source: arXiv:2301.13654 source file (2023-01-31)
Supplement: Supplementary file 10 [file appendixSpecial.tex]

\section{Proofs Omitted from Section~\ref{sec:easy} }\label{sec:app_easy}

\convex*

\begin{proof}
	Let $\zvec^\prime$ and $\zvec^{\prime\prime}$ be Constrained $\epsilon$-Phi-equilibria that is for all $i\in[N]$:
	\[
	\epsilon+u_i(\zvec^\prime)\ge u_i(\phi_i^\prime\diamond\zvec^\prime)
	\]
	for $\phi^\prime\in\arg\max\limits_{\phi_i\in\Phi^\mcS_i}u_i(\phi_i\diamond\zvec^\prime)$. Equivalently it holds for all $i\in[N]$ that:
	\[
	\epsilon+u_i(\zvec^{\prime\prime})\ge u_i(\phi_i^{\prime\prime}\diamond\zvec^{\prime\prime})
	\]
	where $\phi^{\prime\prime}\in\arg\max\limits_{\phi_i\in\Phi^\mcS_i}u_i(\phi_i\diamond\zvec^{\prime\prime})$.
	For any $\zvec:=\alpha \zvec^\prime+(1-\alpha)\zvec^{\prime\prime}$ we have that:
	\begin{align*}
	\epsilon+u_i(\zvec)&=\alpha\left(\epsilon+ u_i(\zvec^\prime)\right)+(1-\alpha)\left(\epsilon+u_i(\zvec^{\prime\prime})\right)\\
	&\ge\alpha u_i(\phi_i^\prime\diamond\zvec^\prime)+(1-\alpha)u_i(\phi_i^{\prime\prime}\diamond\zvec^{\prime\prime})\\
	&\ge\max\limits_{\phi_i\in\Phi_i^\mcS} u_i(\phi_i\diamond\zvec),
	\end{align*}
	where the inequality holds for the linearity of $u_i$, the first inequality as both $\zvec^\prime$ and $\zvec^{\prime\prime}$ are Constrained $\epsilon$-Phi-equilibria and the last inequality holds since the $\max$ is a convex operator.
\end{proof}


\optimalsimple*

\begin{proof}
	%
	\textsc{ApxCPE}$(1,0)$ amounts to solving the following problem:
	%
	\begin{subequations}
		\begin{align}
		\max\limits_{\zvec\in\mcS} & \,\, \ell(\zvec) \quad \text{s.t.}  \\
		& u_i(\zvec) \ge \max_{\phi_i\in\Phi_i^\mcS} u_i(\phi_i\diamond \zvec) \quad \forall i\in \N,
		\end{align}
	\end{subequations}
	which can be written as an LP with (possibly) exponentially-many constraints, by writing a constraint for each vertex of $\Phi_i^\mcS$.
	%
	We can find an exact solution to such an LP in polynomial time by means of the ellipsoid algorithm that uses suitable separation oracle.
	%
	Such an oracle solves the following optimization problem for every $i\in \N$:
	%
	\[
		\phi_i^\star\in\arg\max_{\phi_i\in\Phi_i^\mcS} u_i(\phi_i\diamond \zvec).
	\]
	%
	Then, the oracle returns as a separating hyperplane the incentive constraint corresponding to a $\phi_i^\star$ (if any) such that $u_i(\zvec)\ge u_i(\phi_i^\star\diamond \zvec)$.
	%
	Since all the steps of the separation oracle can be implemented in polynomial time, the ellipsoid algorithm runs in polynomial time, concluding the proof.
	%
\end{proof}


\learning*



\begin{proof}
	Any regret minimizer $\mfR_i$ for $\Phi_i^\mcS$ guarantees that, for every $\phi_i \in \Phi_i^\mcS$:
	%
	\begin{equation}\label{eq:regret1}
	\sum\limits_{t=1}^T u_i(\phi_i\diamond\zvec_t)- \sum\limits_{t=1}^T u_i(\phi_{i,t}\diamond\zvec_t) \le \epsilon_{i,T} \, T,
	\end{equation}
	%
	where $\epsilon_{i,T}=o(T)$.
	%
	Since $\xvec_{i,t}[a]=\sum_{b \in \A_i}\phi_{i,t}[b,a]\xvec_{i,t}[b]$ for all $ a\in\A_i$, for every $t \in [T]$ and $\avec = (a_i, \avec_{-i}) \in \A$:
	%
	\begin{align*}\label{eq:fixedpoint}
	(\phi_{i,t}\diamond\zvec_t)[a_i,\avec_{-i}] &= \sum\limits_{b\in\A_i}\phi_{i,t}[b,a_i]\zvec[b,\avec_{-i}]\\
	&=\sum\limits_{b\in\A_i}\phi_{i,t}[b,a_i]\Big(\xvec_{i,t}[b]\otimes\xvec_{-i,t}[\avec_{-i}]\Big)\\
	&=\left(\sum\limits_{b\in\A_i}\phi_{i,t}[b,a_i]\xvec_{i,t}[b]\right)\otimes\xvec_{-i,t}[\avec_{-i}]\\
	&=\xvec_{i,t}[a_i]\otimes\xvec_{-i,t}[\avec_{-i}]\\
	&=\zvec_t[a_i,\avec_{-i}],
	\end{align*}
	%
	Plugging the equation above into Equation~\eqref{eq:regret1}, we get:
	\[
	\sum\limits_{t=1}^T u_i(\phi_i\diamond\zvec_t)- \sum\limits_{t=1}^T u_i(\zvec_t) \le \epsilon_{i,T} \, T.
	\]
	Now, since $\bar\zvec_T:=\sum_{t=1}^T\zvec_t$ and $u_i(\zvec)$ is linear in $\zvec$, we can conclude that, for every $i\in \N$ and $\phi_i \in \Phi_i^\mcS$:
	\[
	u_i(\zvec_T)\ge u_i(\phi_i\diamond\bar\zvec_T) - \epsilon_{i,T},
	\]
	and, thus, by letting $\epsilon_{T} := \max_{i \in \N}\epsilon_{i,T}$ we get that $\bar\zvec_T$ satisfies the incentivize constrained for being a constrained $\epsilon_{T}$-Phi-equilibrium.
	%
	%is a constrained $(\epsilon_{T})$-Phi-equilibrium.
	%
	We are left to verify that $\bar\zvec_T\in\mcS$, namely $\cvec_i(\bar\zvec_T)\le \zerovec$ for all $i\in \N$.
	%
	This readily proved as:
	%
	\begin{align*}
	\cvec_i(\bar\zvec_T)&=\frac{1}{T}\sum\limits_{t=1}^T\cvec_i(\zvec_t)\\
	&=\frac{1}{T}\sum\limits_{t=1}^T\cvec_i(\phi_{i,t}\diamond\zvec_t)\\
	&=\frac{1}{T}\sum\limits_{t=1}^T\tilde\cvec_i(\phi_{i,t})\\
	&\leq \zerovec,
	\end{align*}
	%
	where the first equality holds since $\cvec_i$ is linear, the second equality holds thanks to $\zvec_t = \phi_{i,t}\diamond\zvec_t$, the third one by Assumption~\ref{ass:cce}, while the inequality holds since $\phi_{i,t}\in\Phi_i^\mcS$.
	%
	This concludes the proof of the first part of the statement.
	
	
	In conclusion, Algorithm~\ref{alg:noregret} runs in polynomial time as finding $\xvec_{i,t}[a]=\sum_{b\in\A_i}\phi_{i,t}[b,a_i]\xvec_{i,t}[b]$ for all $a \in\A_i$ is equivalent to finding a stationary distribution of a Markov Chain, which can be done in polynomial time.
	%
	Moreover, we can implement the regret minimizers $\mfR_i$ over the polytopes $\Phi_i^\mcS$ so that their operations run in polynomial time, such as, \emph{e.g.}, \emph{online gradient descent}; see~\citep{hazan2016introduction}.
	%
	% it is well known that there exists no-regret algorithms $\mfR_i$ over polytopes that run in polynomial time in the dimension of the set $\Phi_i$.
	%
	%	We are left to verify that $\bar\zvec_T\in\mcS$, \ie $\Cvec_i(\bar\zvec_T)\le0$ for all $i\in[N]$. Consider the following chain of equations:
	%	%
	%	\begin{align*}
	%		\Cvec_i(\bar\zvec_T)&:=\frac{1}{T}\sum\limits_{t=1}^T\Cvec_i(\zvec_t)\\
	%		&=\frac{1}{T}\sum\limits_{t=1}^T\Cvec_i(\phi_{i,t}\diamond\zvec_t)\\
	%		&=\frac{1}{T}\sum\limits_{t=1}^T\tilde\Cvec_i(\phi_{i,t})\le0,
	%	\end{align*}
	%	%
	%	where the first equality holds since $\Cvec_i$ is linear, the second equality holds thanks to Equation~\ref{eq:fixedpoint}. Then we used that Assumption~\ref{ass:cce} and that $\phi_{i,t}\in\Phi_i^\mcS$.
	%	%
\end{proof}



\marginal*

\begin{proof}
	Since the costs $\cvec_i(\avec)$ of player $i \in \N$ only depends on player $i$'s action $a_i$ and \emph{not} on the actions of other players, it is possible to show that there exists $\tilde \cvec_i: \Phi_{\textnormal{CCE}}\to [-1,1]^m$ such that the following holds for every $\zvec \in \Delta_{\A}$:
	%
	\begin{align*}
	\tilde\cvec_i(\phi_i) := \cvec_i(\phi_i\diamond\zvec).
	\end{align*}
	%
	Indeed, for every $\phi_i \in \Phi_{\textnormal{CCE}}$, by definition of $\Phi_{\textnormal{CCE}}$ there exists a probability distribution $\boldsymbol{h} \in \Delta_{\A_i}: \phi_i[b,a]=\boldsymbol{h}[a]$ for all $b,a\in\A_i$.
	%
	Then, for every $a_i \in \A_i$ and $\avec_{-i} \in \A_{-i}$, we can write:
	\begin{align*}
	(\phi_i\diamond \zvec)[a_i,\avec_{-i}] &= \sum_{b\in\A_i}\phi_i[b,a_{i}]\zvec[b,\avec_{-i}] \\
	& = \sum_{b\in\A_i}\boldsymbol{h}[a_i]\zvec[b,\avec_{-i}] \\
	& = \boldsymbol{h}[a_i] \sum_{b\in\A_i}\zvec[b,\avec_{-i}].
	\end{align*}
	%
	Moreover, it holds:
	%
	\begin{align*}
	\cvec_i (\phi_i\diamond \zvec)[a_i,\avec_{-i}] & = \sum_{\avec \in \A} \cvec_i(\avec) (\phi_i\diamond \zvec)[a_i,\avec_{-i}] \\
	& = \sum_{\avec \in \A} \cvec_i(\avec) \boldsymbol{h}[a_i] \sum_{b\in\A_i}\zvec[b,\avec_{-i}] \\
	& = \sum_{a_i \in \A_i} \cvec_i(a_i,\cdot) \boldsymbol{h}[a_i] \sum_{\avec_{-i} \in \A_{-i}}\sum_{b\in\A_i}\zvec[b,\avec_{-i}]\\
	& = \sum_{a_i \in \A_i} \cvec_i(a_i,\cdot) \boldsymbol{h}[a_i] ,
	\end{align*}
	which only depends on $\phi_i$, as desired.
	%
	Notice that, in the equations above, for every $a \in \A_i$ we let $\cvec_i(a,\cdot)$ be the (unique) value of $\cvec_i(\avec)$ for all $\avec \in \A: a_i = a$.
	%
	% Since $\Cvec_i(\zvec)$ only depends on the marginalization of the $i$-th player we can write that:
	%
	%	\begin{align}
	%		\cvec_i(\phi_i\diamond\zvec) = \tilde\cvec^\prime_i(\tilde\xvec^{\phi_i}_i),
	%	\end{align}
	%	where $\tilde\xvec_i$ is the marginalized strategy obtained after deviation $\phi_i$, \ie $\tilde\xvec^{\phi_i}_i[a_i]:=\sum_{b\in\A^i}\phi_i[b,a_i]\xvec_i(b)$. Now, if $\phi_i\in\Phi_{i,,\textnormal{CCE}}$ we know it exists a probability vector $\cvec\in\Delta(\A_i)$ such that $\phi_i[b,a_i]=\cvec[a_i]$ for all $b,a_i\in\A^i$. Thus $\tilde\xvec^{\phi_i}_i$ becomes:
	%	\[
	%	\tilde\xvec^{\phi_i}_i[a_i]:=\sum_{b\in\A^i}\phi_i[b,a_i]\xvec_i(b)=\sum_{b\in\A^i}\cvec[a_i]\xvec_i(b) = \cvec[a_i]
	%	\]
	%	and thus $\Cvec_i(\phi_i\diamond\zvec)$ only depends on $\phi_i$ and Assumption~\ref{ass:cce} is verified.
\end{proof}
